# Supplementary material for: Finding Favourite Tuples on Data Streams with Provably Few Comparisons
Source: arXiv:2307.02946 source file (2023-07-06)
Supplement: Supplementary file 1 [file supp-backup-QP.tex]

%\section{Another filter for \irm with ties}
%\label{se:backup}

\input{alg-robust-backup}

In \cref{alg:robust-backup}, we provide a filter to handle ties under \cref{asm:dirm},
which is easier to analyze but has a worse guarantee on the query complexity.
We maintain a totally sorted subset $R$ of ``representatives'' in a sample set $S$.
For each representative $\vecy \in R$, we create a group $G_\vecy$.
When given a new tuple \vecx, we sort \vecx into $R$ if no tie is encountered.
Otherwise, we add \vecx into every group $G_\vecy$ such that $\vecx \cmp \vecy$.
Note that there are at most two such groups for any \vecx.
Besides, tuple \vecx is compared with every tuple in $G_\vecy$, and all comparable pairs are kept in an additional set $P_\vecx$.
In the end, the best tuple in $R$ will be returned.

To see whether a filter in \cref{alg:robust-backup} can prune a given tuple \vecx, we test the following condition.
Let $R = \{ \vecx_1, \ldots \}$ where $\vecx_1$ is the top tuple.
A tuple \vecx can be pruned if 
there exists $\vecx'$ such that $\norm{\vecx - \vecx'}_2 \le \Creg$, where
\begin{align}
	\vecx' = 
	\sum_{\vecy \in G_{\vecx_1}} \nu_\vecy \, \vecy  
	&+ \sum_{j=1} \sum_{(\vecw,\vecz) \in G_{\vecx_{j+1}} \setminus G_{\vecx_j} \times G_{\vecx_j} \setminus G_{\vecx_{j+1}}} \alpha_{\vecw,\vecz} (\vecw - \vecz) \nonumber \\
	&+ \sum_{\vecy \in S} \sum_{(\vecw,\vecz) \in P_\vecy} \alpha_{\vecw,\vecz} (\vecw - \vecz) \label{eq:filter-robust-backup}\\
	&\text{such that} 
	\sum_{\vecy \in G_{\vecx_1}} \nu_\vecy = 1 \text{ and all } \nu, \alpha \ge 0 \nonumber .
\end{align}
The idea is similar to \cref{eq:filter}, except that 
the top tuple $\vecx_1$ in \cref{eq:filter} is replaced by an aggregated tuple by convex combination, and
every pair difference $\vecx_{j+1} - \vecx_{j}$ is replaced by pair differences between two groups.
In addition, pair differences within a group is are handled by the last term.
\note{
Every immediate comparable pair is included in \cref{eq:filter-robust-backup}, where 
a pair $\vecx,\vecy \in S$ with $\util(\vecx) < \util(\vecy)$ is called immediate if there is no $\vecz \in S$ such that $\util(\vecx) < \util(\vecz) < \util(\vecy)$ and all three are comparable.
To see this, discuss two cases, $\vecx,\vecy$ in one group and in two different groups.
}
We write 
\begin{align}
	S \infersim \vecx \label{eq:implies-robust-backup},
\end{align}
if the above condition can be met.

The number of comparisons that is needed by \cref{alg:robust-backup} depends on the actual input,
specifically, the largest size of any pairwise \vecu-similar subset of~\D.
\begin{theorem}
\label{thm:num_of_S-robust-backup}
Assume $\epsilon > 0$ and let $\nD = |\D|$ be the size of data.
Let $c = \util(\vecx^*) \in [0,1]$ be the utility of the best tuple~$\vecx^*$.
Under \cref{asm:dirm},
with a pool size $\nPl = \ceil{64 \ln 2\nD}$,
\cref{alg:framework,alg:robust-backup} return an $(\Creg/c + 2\Ccmp)$-regret tuple for the \irm problem.

Let $\infd = \Cinfd$, where
$d$ is the intrinsic dimension of~\D, and
\Ccmpmax be the largest size of a pairwise \vecu-similar subset of \D.
Then, with probability at least $1-1/\nD$, at most
\[
	\bigO(\log(\nD) \, 8 \infd \Ccmpmax (\log(8 \infd \Ccmpmax) + 4\Ccmpmax)) + \nPl
\]
comparisons
are made.
\end{theorem}


In the rest of this section, we prove \cref{thm:num_of_S-robust-backup}.


\subsection{Proofs}

The proof is similar to that of \cref{thm:num_of_S},
except that we need a new proof for \cref{lemma:4t},
since in the presence of ties, we may not be able to totally sort a sample $S$.
Instead, we show that a partially sorted set $S$ of a sufficient size can also be effective in pruning.

\begin{lemma}
\label{lemma:4t-robust-backup}
Under \cref{asm:dirm},
given a set $S \subseteq \X$ of size $8\infd \Ccmpmax$,
we have
\[
	|\{ \vecx \in S: S-\vecx \infersim \vecx \}| \ge \frac34 |S|,
\]
where $\infd = \Cinfd$, 
and \Ccmpmax is the largest size of a pairwise \vecu-similar subset of \X. 
\end{lemma}
\begin{proof}
Note that by the definition of \Ccmpmax, 
for any particular tuple $\vecx \in S$,
there are at most $2(\Ccmpmax-1)$ tuples that are \vecu-similar with tuple \vecx.
Hence, given a set $T$ of size $2\infd \Ccmpmax$, 
it is always possible to identify a totally sorted list $L$ of length at least $\infd$.
Notice that \cref{eq:filter-robust-backup} is a generalization of \cref{eq:comb} in the presence of ties, and
a form of \cref{eq:comb} using tuples in $L$ is always realizable by \cref{eq:filter-robust-backup}.
Thus, to prune at least 3/4 fraction of $S$, 
one repeatedly finds such a totally sorted list from $S$ and applies \cref{lemma:comb} to prune a tuple in the list
until only $2\infd \Ccmpmax$ tuples remain.
\end{proof}

Denote by $\filtersim(S)$ the set of tuples that can be pruned by $S$, that is,
\begin{align}
	\filtersim(S) = \{ \vecx \in \reals^d: S \infersim \vecx \}.
\end{align}
The proof of the following lemma is identical to that of \cref{lemma:filter}, 
by replacing $\filter(S)$ with $\filtersim(S)$, and 
\cref{lemma:4t} with \cref{lemma:4t-robust} in the reasoning.
\begin{lemma}
\label{lemma:filter-robust-backup}
Given a set of tuples \X, and
a random sample set $S \subseteq \X$ of size $16\infd \Ccmpmax$,
which is added into a filter in \cref{alg:robust-backup},
we have
\[
	\expect \left[ |\filtersim(S) \cap \X| \right] 
	\ge \frac34 |\X|,
\]
where $\infd = \Cinfd$, 
and \Ccmpmax is the largest size of a pairwise \vecu-similar subset of \X. 
Moreover, the expectation is taken over the random choice of~$S$.
\end{lemma}

\begin{proof}[Proof of \cref{thm:num_of_S-robust-backup}]
The proof is similar to \cref{thm:num_of_S} on a high level.
We only elaborate on their differences.

We first prove the guarantee on the regret.
There are two ways we may discard a good tuple \vecx,
either by pruning or because \vecx is \vecu-similar to some tuple when we look for the best tuple in our samples.
By \cref{thm:anytime}, we know that the regret due to pruning is at most $\Creg/c$.
The regret due to \vecu-similarity is at most $2\Ccmp$,
as we lose one \Ccmp in finding the best tuple in each filter, and another \Ccmp in returning the final best tuple.
Thus, the regret is at most $\Creg/c + 2\Ccmp$.

It is identical to \cref{thm:num_of_S} about
how to upper bound the size of every sample and the number of samples,
by replacing \cref{lemma:filter} with \cref{lemma:filter-robust-backup}.
Hence, with probability at least $1-1/\nD$,
it is sufficient to use $\ceil{\log(\nD)}$ sample sets, each with a size $8\infd \Ccmpmax$.

Building one filter requires at most $8\infd \Ccmpmax (\ceil{\log(8\infd \Ccmpmax)} + 4 \Ccmpmax)$ comparisons, because
sorting an new tuple \vecx within $R$ by binary search costs at most $\ceil{\log(8\infd \Ccmpmax)}$, and
comparing \vecx with tuples from at most two groups $G_\vecy$ such that $\vecy \cmp \vecx$ costs $4 \Ccmpmax$.
Finally, finding the best tuple among all filters and the pool requires additional $\nPl + \ceil{\log(\nD)}$ comparisons.
\end{proof}
